# Supplementary material for: Search for exotic spin-dependent interactions using polarized helium
Source: arXiv:2002.02495 source file (2020-03-02)
Supplement: Supplementary file 1 [file appendix.tex]

\section{Appendix}
\begin{align}
    p & = 1,\\
    n_s &= 2.4\times 10^{25} \text{m}^{-3},\\
    \mu_3 &= 1.07\times 10^{-26} \text{J}/\text{T},\\
    \gamma_3 &= 2\pi\times 32.4\times 10^{6} \text{Hz/T},\\
    T_2 &= 1000 \text{s},\\
    \mu_0 & = 4\pi\times 10^{-7} \text{N}/\text{A}^2
\end{align}
\begin{align}
    \mu_0 M &= \frac{\mu_0}{2}pn_s\mu_3\gamma_3 B_\text{eff}T_2 = 10^{-15} \text{T}\\
    B_\text{eff} &=  10^{-15}/ (\frac{\mu_0}{2}pn_s\mu_3\gamma_3 B_\text{eff}T_2)\\
    &=3\times 10^{-20} \text{T}
\end{align}
